# Supplementary material for: Adaptive-SpikeNet: Event-based Optical Flow Estimation using Spiking Neural Networks with Learnable Neuronal Dynamics
Source: arXiv:2209.11741 source file (2023-03-14)
Supplement: Supplementary file 1 [file appendix.tex]

\section*{APPENDIX}
